# Supplementary material for: UnifiedSKG: Unifying and Multi-Tasking Structured Knowledge Grounding with Text-to-Text Language Models
Source: arXiv:2201.05966 source file (2022-10-18)
Supplement: Supplementary file 6 [file multitask.tex]

% Mention upsampling in the main paper. 
%\section{Multi-Task Learning Baseline}
%\label{app:multi-task}

\iffalse
\paragraph{Task Pairs}
We studied a diverse set of task combinations as follows.
1) \textit{Similar tasks} (e.g., Spider and CoSQL both translate natural language requests into SQLs).
2) \textit{Parallel tasks} (e.g., Spider and GrailQA are both semantic parsing, while they have different structured knowledge (database and knowledge graph) and different output (SQL and s-Expression)).
3) \textit{Subtask} (e.g., question answering can be viewed as the execution semantic parses). 
4) \textit{Inverse tasks} (e.g., Spider translates natural language questions into SQLs, and SQL2Text translates SQLs into natural language questions). 
5) \textit{Similar output, different input} (e.g., SQL2Text and Logic2Text both translate formal language to natural language, while SQL2Text takes SQLs as input and Logic2Text takes logical expressions as input).
6) \textit{Similar input, different output} (e.g., FeTaQA and WikiTQ both take tables as input, while FeTaQA outputs free-form answers and WikiTQ outputs answer sets). 
%\chen{as discussed on Nov 4, we should give reasons for the choice. If resources are available, both directions should be studied. } 

\input{tables/multi_task_all_tasks}

\fi
